# Supplementary material for: Experimental Evidence of Stable 2$H$ Phase on the Surface of Layered 1$T'$-TaTe$_2$
Source: arXiv:2009.00987 source file (2020-12-22)
Supplement: Supplementary file 1 [file TT_ACS_Supple.pdf]

Supporting Information for:

# Experimental Evidence of Stable $2H$ Phase on the Surface of Layered $1T'$-TaTe$_2$

Indrani Kar,[†] Kapildeb Dolui,[‡] Luminita Harnagea,[¶] Yevhen Kushnirenko,[§] Grigory Shipunov,[§] Nicholas C. Plumb,[‖] Ming Shi,[‖] Bernd Büchner,[§] and Setti Thirupathaiah[*,†]

†*Department of Condensed Matter Physics and Material Sciences, S N Bose National Centre for Basic Sciences, Kolkata, West Bengal-700106, India*

‡*Department of Physics and Astronomy, University of Delaware, Newark, DE 19716, USA*

¶*Indian Institute of Science Education and Research, Dr. Homi Bhabha Road, Pune, Maharashtra-411008, India*

§*Leibniz-Institute for Solid State and Materials Research Dresden, P.O.Box 270116, D-01171 Dresden, Germany*

‖*Swiss Light Source, Paul Scherrer Institute, CH-5232 Villigen PSI, Switzerland*

E-mail: setti@bose.res.in

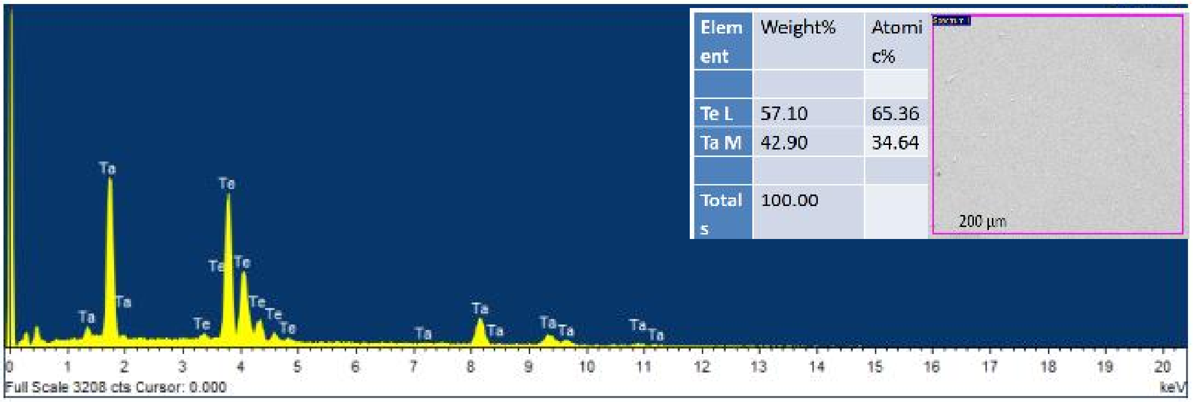


**Figure 1:** Energy dispersive X-ray spectroscopy (EDX) measurement on $1T'$-$TaTe_2$ single crystal. Atomic and weight percentage, scanning electron microscope image of the area are given in the inset.

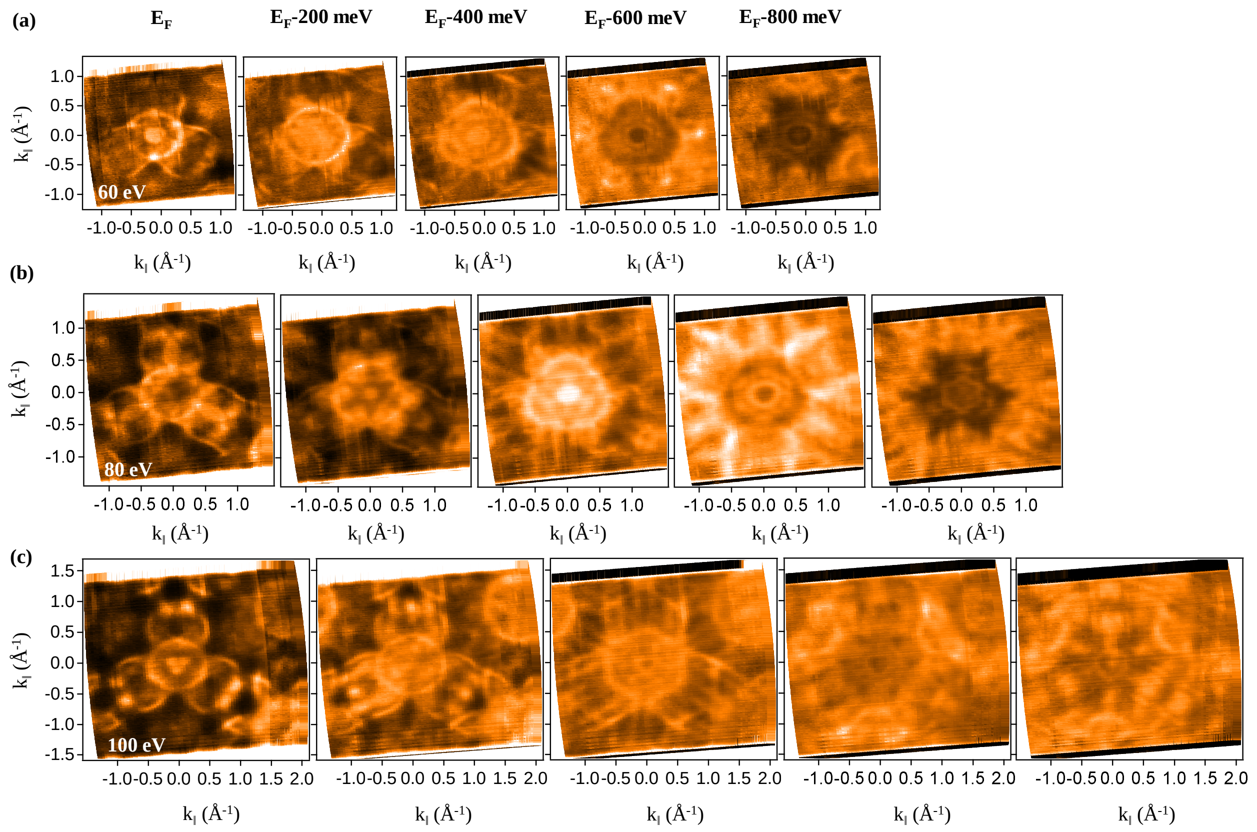


**Figure 2:** Constant energy contours of $TaTe_2$ measured at 1 K using $p$ polarized light with photon energies of (a) 60 eV, (b) 80 eV, and (c) 100 eV at Fermi level and at binding energies $E_B = 200$, 400, 600 and 800 meV from left to right.

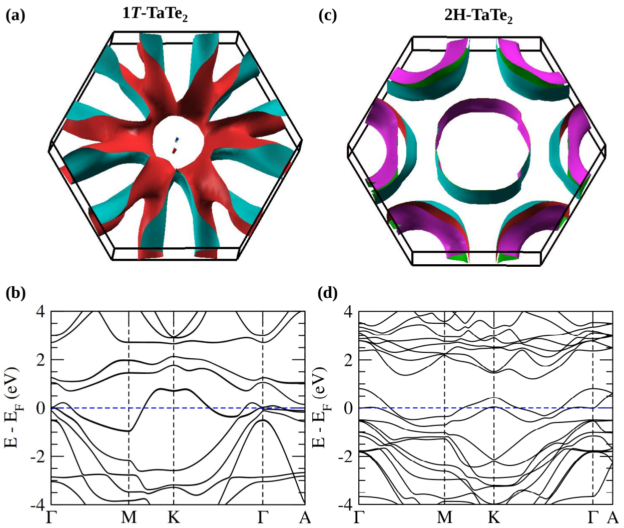


**Figure 3:** (a) 3D view of the calculated Fermi surface topology of bulk 1$T$-$TaTe_2$. (b) Electronic band structure of bulk 1$T$-$TaTe_2$. (c) 3D view of the calculated Fermi surface topology of bulk 2$H$-$TaTe_2$. (d) Electronic band structure of bulk 2$H$-$TaTe_2$
